# Supplementary material for: Balancing Statistical and Computational Precision: A General Theory and Applications to Sparse Regression
Source: arXiv:1609.07195 source file (2022-09-14)
Supplement: Supplementary file 1 [file suppl_exp.tex]

\section*{Appendix D. Additional simulation results}

We provide additional simulation results to complement the empirical studies in the main part of the paper. We consider the $n=500$ and $p=1000$ setting with the specifications as described in the main part of the paper - except for the stated differences.

In Table~\ref{tabadd}, we add the results for Lasso with AIC and BIC. In Table~\ref{tabS}, we consider different support sizes. In Table~\ref{tabr}, we vary the correlation.

The BIC and AIC criteria are defined as in~\cite{Zou07}:
\begin{align*}
    \text{BIC}(\tuningparameter) &= \frac{\normtwo{Y-X\cm^{\tuningparameter}}^2}{\nobs\sigma^2_\varepsilon}+\frac{\log(\nobs)|\settilde^{\tuningparameter}|}{\nobs}\\
    \text{AIC}(\tuningparameter) &= \frac{\normtwo{Y-X\cm^{\tuningparameter}}^2}{\nobs\sigma^2_\varepsilon}+\frac{2|\settilde^{\tuningparameter}|}{\nobs}\,,
\end{align*}
where $\sigma^2_\varepsilon$ is the variance of the noise $\varepsilon$. In our experiments, $\sigma^2_\varepsilon=1$. To establish valid comparisons, we again implement these schemes with the \texttt{SPAMS} package.

\begin{table}%[!ht]
  \centering
  %\vspace{.5\baselineskip}
%   \fbox{
  \begin{tabular}{lll}
    \toprule
    % & \multicolumn{2}{c}{$|\sets|=5$} & \multicolumn{2}{c}{$|\sets|=30$}                  \\
    % \cmidrule{2-3}
    Method     & Timing     & Hamming distance \\
    % \midrule
    \hline
    \lcvs & $137.15\pm 9.33$  &  $56.00\pm 18.37$  \\
    \lcvg     & $~~~2.08\pm 0.32$ & $44.90\pm 16.07$ \\
    \lbics     & $~\,20.12\pm 5.98$ & $10.40\pm ~\,7.15$  \\
    \laics     & $~\,20.12\pm 5.98$ & $45.30\pm21.40$\\
    FOS     & $~~\,\,0.10\pm 0.06$       & $~\,8.60\pm~\,3.10$\\
    \bottomrule
  \end{tabular}
%   }
\caption{\label{tabadd}Average run times (in seconds) and average Hamming distances for \lcvs, \lcvg, \lbics, \laics, and FOS.}
\end{table}

\begin{table}%[!ht]
\centering
%  \vspace{.5\baselineskip}
% \fbox{
  \begin{tabular}{lllll}
    \toprule
    & \multicolumn{2}{c}{$|\sets|=5$} & \multicolumn{2}{c}{$|\sets|=30$}                  \\
%    \cmidrule{2-5}
	\cline{2-5}
    Method     & Timing     & Hamming distance & Timing     & Hamming distance\\
%    \midrule
	\hline
    \lcvs & $283.19\pm 75.41$  &  $43.50\pm 19.53$  & $224.92\pm 41.77$  &$117.50\pm 22.49$\\
    \lcvg     & $~~~2.59\pm~\,0.40$ & $29.90\pm 12.66$    & $~~~2.52\pm~~0.25$ & $~\,98.00\pm 35.50$  \\
    FOS     & $~~~0.76\pm~\,2.13$       & $~\,4.40\pm~\,1.58$ & $~~~2.23\pm~~2.01$      & $~\,20.60\pm 11.98$ \\
    \bottomrule
  \end{tabular}
%   }
  \caption{Average run times (in seconds) and average Hamming distances for \lcvs, \lcvg, and FOS for two different sizes of the true support: $|\sets|\in\{5,30\}$. \label{tabS}}
\end{table}

\begin{table}%[!ht]
  \centering
%  \vspace{.5\baselineskip}
% \fbox{
  \begin{tabular}{lllll}
    \toprule
    & \multicolumn{2}{c}{$\rho=0$} & \multicolumn{2}{c}{$\rho=0.4$}                  \\
%    \cmidrule{2-5}
	\cline{2-5}
    Method     & Timing     & Hamming distance & Timing     & Hamming distance\\
%    \midrule
	\hline
    \lcvs & $168.03\pm 25.28$  &  $56.50\pm 22.45$  & $177.79\pm 48.11$  & $58.30\pm 20.67$\\
    \lcvg     & $~~~2.46\pm~\,0.24$ & $40.40\pm 13.17$    & $~~~2.36\pm~\,0.21$ & $44.50\pm 18.12$  \\
    FOS     & $~~~1.78\pm~\,0.73$       & $~\,1.10\pm~\,1.29$ & $~~~0.12\pm~\,0.06$      & $~\,9.70\pm~\,0.95$ \\
    \bottomrule
  \end{tabular}
%  } 
\caption{Average run times (in seconds) and average Hamming distances for \lcvs, \lcvg, and FOS for two different strengths of the pairwise correlations: $\rho\in\{0,0.4\}$. \label{tabr}}
  \end{table}
